# Supplementary material for: Logical Consistency and Greater Descriptive Power for Facial Hair Attribute Learning
Source: arXiv:2302.11102 source file (2023-04-16)
Supplement: Supplementary file 2 [file sup_mat_accuracy.tex]

\begin{table}[t]
\centering
\begin{tabular}{cccccc|c|c|c|c|c|c}
\hline
\multicolumn{1}{c|}{} &
  \multicolumn{1}{c|}{\rotatebox{90}{Clean Shaven}} &
  \multicolumn{1}{c|}{\rotatebox{90}{Chin Area}} &
  \multicolumn{1}{c|}{\rotatebox{90}{Side to Side}} &
  \multicolumn{1}{c|}{\rotatebox{90}{Beard area Info Not Vis}} &
  \rotatebox{90}{5 O'clock Shadow} &
  \rotatebox{90}{Short} &
  \rotatebox{90}{Medium} &
  \rotatebox{90}{Long} &
  \rotatebox{90}{Bread length Info Not Vis} &
  \rotatebox{90}{Mustache-None} &
  \rotatebox{90}{Mustache-Isolated} \\ \hline
\multicolumn{1}{c|}{Overall acc} &
  \multicolumn{1}{c|}{86.86} &
  \multicolumn{1}{c|}{87.46} &
  \multicolumn{1}{c|}{88.05} &
  \multicolumn{1}{c|}{92.28} &
  80.62 &
  83.44 &
  92.40 &
  96.75 &
  91.34 &
  86.26 &
  85.74 \\
\multicolumn{1}{c|}{Negative acc} &
  \multicolumn{1}{c|}{93.88} &
  \multicolumn{1}{c|}{91.41} &
  \multicolumn{1}{c|}{88.34} &
  \multicolumn{1}{c|}{96.11} &
  80.62 &
  94.32 &
  98.04 &
  97.27 &
  94.36 &
  91.24 &
  90.27 \\
\multicolumn{1}{c|}{Positive acc} &
  \multicolumn{1}{c|}{70.21} &
  \multicolumn{1}{c|}{71.14} &
  \multicolumn{1}{c|}{87.59} &
  \multicolumn{1}{c|}{76.05} &
  80.61 &
  55.42 &
  23.60 &
  78.81 &
  78.18 &
  77.36 &
  66.42 \\ \hline
 &
   &
   &
   &
   &
   &
   &
   &
   &
   &
   &
   \\ \hline
\multicolumn{1}{c|}{} &
  \multicolumn{1}{c|}{\rotatebox{90}{Mustache Connected to Beard}} &
  \multicolumn{1}{c|}{\rotatebox{90}{Mustache Info Not Vis}} &
  \multicolumn{1}{c|}{\rotatebox{90}{Sideburns-None}} &
  \multicolumn{1}{c|}{\rotatebox{90}{Sideburns-present}} &
  \rotatebox{90}{Sideburns Connected to Beard} &
  \rotatebox{90}{Sideburns Info Not Vis} &
  \rotatebox{90}{Bald False} &
  \rotatebox{90}{Bald Top Only} &
  \rotatebox{90}{Bald Top and Sides} &
  \rotatebox{90}{Bald Sides Only} &
  \rotatebox{90}{Bald Info Not Vis} \\ \hline
\multicolumn{1}{c|}{Overall acc} &
  \multicolumn{1}{c|}{89.11} &
  \multicolumn{1}{c|}{93.11} &
  \multicolumn{1}{c|}{80.33} &
  \multicolumn{1}{c|}{86.05} &
  89.86 &
  88.94 &
  92.80 &
  95.46 &
  97.37 &
  98.57 &
  95.79 \\
\multicolumn{1}{c|}{Negative acc} &
  \multicolumn{1}{c|}{91.15} &
  \multicolumn{1}{c|}{94.75} &
  \multicolumn{1}{c|}{87.17} &
  \multicolumn{1}{c|}{88.61} &
  93.25 &
  92.39 &
  84.00 &
  96.44 &
  98.58 &
  98.96 &
  97.25 \\
\multicolumn{1}{c|}{Positive acc} &
  \multicolumn{1}{c|}{85.64} &
  \multicolumn{1}{c|}{74.57} &
  \multicolumn{1}{c|}{70.97} &
  \multicolumn{1}{c|}{70.77} &
  78.46 &
  75.57 &
  95.10 &
  78.17 &
  66.25 &
  0 &
  84.21 \\ \hline
\end{tabular}
\caption{Performance of the BCELoss + LCPLoss + label compensation strategy on the logically inconsistent predictions counted case.}
\label{sup_table:performance}
\end{table}
