# Supplementary material for: Logical Consistency and Greater Descriptive Power for Facial Hair Attribute Learning
Source: arXiv:2302.11102 source file (2023-04-16)
Supplement: Supplementary file 4 [file Beard_Length.tex]

\begin{figure*}[h]
    \centering
    \begin{subfigure}[b]{1\linewidth}
    \captionsetup[subfigure]{labelformat=empty}
        \begin{subfigure}[b]{1\linewidth}
            \begin{subfigure}[b]{1\linewidth}
            \centering
                \begin{subfigure}[b]{0.15\linewidth}
                    \includegraphics[width=\linewidth]{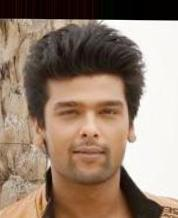}
                    
                \end{subfigure}
                \begin{subfigure}[b]{0.15\linewidth}
                    \includegraphics[width=\linewidth]{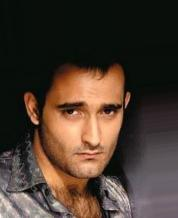}
                    
                \end{subfigure}
                \begin{subfigure}[b]{0.15\linewidth}
                    \includegraphics[width=\linewidth]{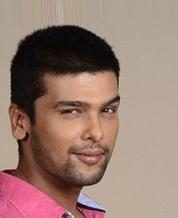}
                    
                \end{subfigure}
                \begin{subfigure}[b]{0.15\linewidth}
                    \includegraphics[width=\linewidth]{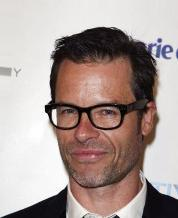}
                    
                \end{subfigure}
                \begin{subfigure}[b]{0.15\linewidth}
                    \includegraphics[width=\linewidth]{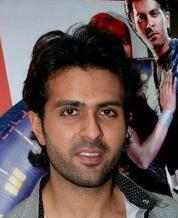}
                    
                \end{subfigure}
                \begin{subfigure}[b]{0.15\linewidth}
                    \includegraphics[width=\linewidth]{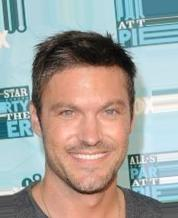}
                \end{subfigure}
            \caption{Samples of the attribute 5 O'clock Shadow.}
            \end{subfigure}
            \begin{subfigure}[b]{1\linewidth}
            \centering
                \begin{subfigure}[b]{0.15\linewidth}
                    \includegraphics[width=\linewidth]{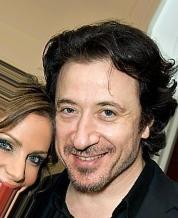}
                    
                \end{subfigure}
                \begin{subfigure}[b]{0.15\linewidth}
                    \includegraphics[width=\linewidth]{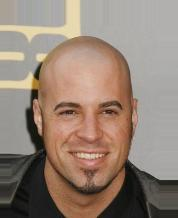}
                    
                \end{subfigure}
                \begin{subfigure}[b]{0.15\linewidth}
                    \includegraphics[width=\linewidth]{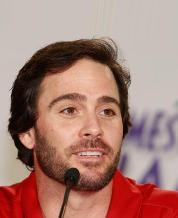}
                    
                \end{subfigure}
                \begin{subfigure}[b]{0.15\linewidth}
                    \includegraphics[width=\linewidth]{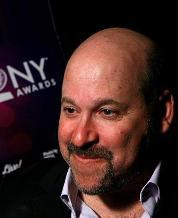}
                    
                \end{subfigure}
                \begin{subfigure}[b]{0.15\linewidth}
                    \includegraphics[width=\linewidth]{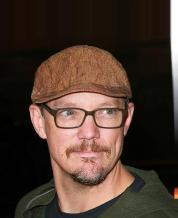}
                    
                \end{subfigure}
                \begin{subfigure}[b]{0.15\linewidth}
                    \includegraphics[width=\linewidth]{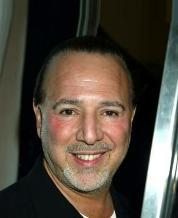}
                    
                \end{subfigure}
            \end{subfigure}
            \caption{Samples of the attribute Short.}
        \end{subfigure}
        
        \begin{subfigure}[b]{1\linewidth}
            \begin{subfigure}[b]{1\linewidth}
            \centering
                \begin{subfigure}[b]{0.15\linewidth}
                    \includegraphics[width=\linewidth]{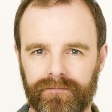}
                    
                \end{subfigure}
                \begin{subfigure}[b]{0.15\linewidth}
                    \includegraphics[width=\linewidth]{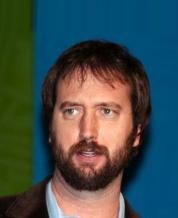}
                    
                \end{subfigure}
                \begin{subfigure}[b]{0.15\linewidth}
                    \includegraphics[width=\linewidth]{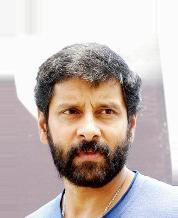}
                    
                \end{subfigure}
                \begin{subfigure}[b]{0.15\linewidth}
                    \includegraphics[width=\linewidth]{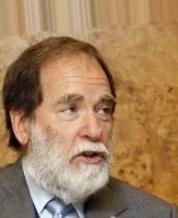}
                    
                \end{subfigure}
                \begin{subfigure}[b]{0.15\linewidth}
                    \includegraphics[width=\linewidth]{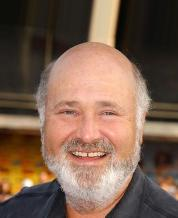}
                    
                \end{subfigure}
                \begin{subfigure}[b]{0.15\linewidth}
                    \includegraphics[width=\linewidth]{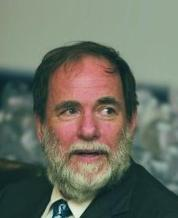}
                \end{subfigure}
            \caption{Samples of the attribute Medium.}
            \end{subfigure}
            \begin{subfigure}[b]{1\linewidth}
            \centering
                \begin{subfigure}[b]{0.15\linewidth}
                    \includegraphics[width=\linewidth]{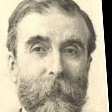}
                    
                \end{subfigure}
                \begin{subfigure}[b]{0.15\linewidth}
                    \includegraphics[width=\linewidth]{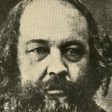}
                    
                \end{subfigure}
                \begin{subfigure}[b]{0.15\linewidth}
                    \includegraphics[width=\linewidth]{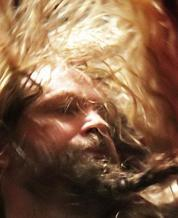}
                    
                \end{subfigure}
                \begin{subfigure}[b]{0.15\linewidth}
                    \includegraphics[width=\linewidth]{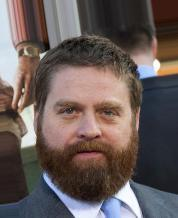}
                    
                \end{subfigure}
                \begin{subfigure}[b]{0.15\linewidth}
                    \includegraphics[width=\linewidth]{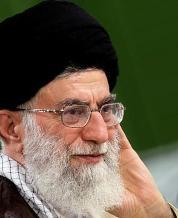}
                    
                \end{subfigure}
                \begin{subfigure}[b]{0.15\linewidth}
                    \includegraphics[width=\linewidth]{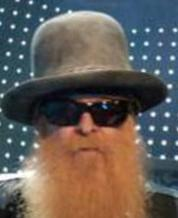}
                \end{subfigure}
            \caption{Samples of the attribute Long.}
            \end{subfigure}
            \begin{subfigure}[b]{1\linewidth}
            \centering
                \begin{subfigure}[b]{0.15\linewidth}
                    \includegraphics[width=\linewidth]{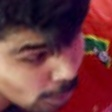}
                    
                \end{subfigure}
                \begin{subfigure}[b]{0.15\linewidth}
                    \includegraphics[width=\linewidth]{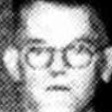}
                    
                \end{subfigure}
                \begin{subfigure}[b]{0.15\linewidth}
                    \includegraphics[width=\linewidth]{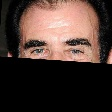}
                    
                \end{subfigure}
                \begin{subfigure}[b]{0.15\linewidth}
                    \includegraphics[width=\linewidth]{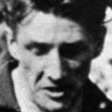}
                    
                \end{subfigure}
                \begin{subfigure}[b]{0.15\linewidth}
                    \includegraphics[width=\linewidth]{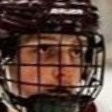}
                    
                \end{subfigure}
                \begin{subfigure}[b]{0.15\linewidth}
                    \includegraphics[width=\linewidth]{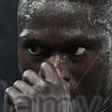}
                \end{subfigure}
            \caption{Samples of the attribute Beard Length Info Not Vis.}
            \end{subfigure}
        \end{subfigure}
    \end{subfigure}
   \caption{Examples of the Beard Length attributes.}
\label{fig:beard_length}
\end{figure*}
