# Supplementary material for: Logical Consistency and Greater Descriptive Power for Facial Hair Attribute Learning
Source: arXiv:2302.11102 source file (2023-04-16)
Supplement: Supplementary file 9 [file sup_mat_consistency_rate.tex]

\begin{table*}[h]
\centering
\begin{tabular}{|l|l|l|l|}
\hline
Attributes                    & Consistency rate
 & Attributes                      & Consistency rate
 \\ \hline
Clean Shaven                 & 0.99                  & Mustache Connected to Beard  & 0.83                 \\ \hline
Chin Area                    & 0.92                  & Mustache Info Not Vis        & 0.99                  \\ \hline
Side to Side                & 0.93                 & Sideburns-None                 & 0.90                 \\ \hline
Beard area Info Not Vis   & 0.98                  & Sideburns-Present              & 0.92                  \\ \hline
5 O'clock Shadow           & 0.91                 & Sideburns Connected to Beard & 0.90                  \\ \hline
Short                         & 0.83                 & Sideburns Info Not Vis       & 0.94                  \\ \hline
Medium                        & 0.89                  & Bald False                     & 0.99                 \\ \hline
Long                          & 1                    & Bald Top Only                       & 0.98                  \\ \hline
Beard length Info Not Vis & 0.98                  & Bald Top and Sides                 & 1                  \\ \hline
Mustache-None                & 0.98                 & Bald Sides Only                     & 1                    \\ \hline
Mustache-Isolated                      & 0.84                 & Bald Info Not Vis            & 0.99                  \\ \hline
\end{tabular}
\caption{The estimated consistency rate of each attribute in the FH37K dataset.}
\label{sup_table:consistency_rate}
\end{table*}
