# Supplementary material for: Logical Consistency and Greater Descriptive Power for Facial Hair Attribute Learning
Source: arXiv:2302.11102 source file (2023-04-16)
Supplement: Supplementary file 10 [file supplemental_material_number_of_samples.tex]

\begin{table*}[h]
\centering
\begin{tabular}{|l|l|l|l|}
\hline
Attributes                    & \# of positive samples & Attributes                      & \# of positive samples \\ \hline
Clean Shaven                 & 9,562                  & Mustache Connected to Beard  & 15,887                 \\ \hline
Chin Area                    & 9,381                  & Mustache Info Not Vis        & 1,343                  \\ \hline
Side to Side                & 17,375                 & Sideburns-None                 & 14,004                 \\ \hline
Beard area Info Not Vis   & 3,001                  & Sideburns-Present              & 7,361                  \\ \hline
5 O'clock Shadow           & 11,759                 & Sideburns Connected to Beard & 9,809                  \\ \hline
Short                         & 11,693                 & Sideburns Info Not Vis       & 6,391                  \\ \hline
Medium                        & 2,475                  & Bald False                     & 31,085                 \\ \hline
Long                          & 747                    & Bald Top Only                       & 1,065                  \\ \hline
Beard length Info Not Vis & 2,757                  & Bald Top and Sides                 & 1,321                  \\ \hline
Mustache-None                & 10,228                 & Bald Sides Only                     & 161                    \\ \hline
Mustache-Isolated                      & 10,107                 & Bald Info Not Vis            & 3,933                  \\ \hline
\end{tabular}
\caption{Statistic information of the FH37K dataset.}
\label{sup_table:number_of_samples}
\end{table*}
