# Supplementary material for: Logical Consistency and Greater Descriptive Power for Facial Hair Attribute Learning
Source: arXiv:2302.11102 source file (2023-04-16)
Supplement: Supplementary file 11 [file Supplemental_material.tex]

\documentclass[10pt,twocolumn,letterpaper]{article}

\usepackage{cvpr}              %

\usepackage[accsupp]{axessibility}  %



\usepackage{graphicx}
\usepackage{amsmath}
\usepackage{amssymb}
\usepackage{booktabs}
\usepackage{xcolor}
\usepackage{algorithm}
\usepackage{algorithmic}
\usepackage{pifont}
\usepackage[utf8]{inputenc}
\usepackage{hhline}
\usepackage{color, colortbl}
\usepackage{multirow}
\usepackage{times}
\usepackage{epsfig}
\usepackage{lipsum} 
\usepackage{pythonhighlight}
\usepackage{makecell}
\usepackage{minted}
\usepackage{url}
\newcommand{\ra}[1]{\renewcommand{\arraystretch}{#1}}
\newcommand{\cmark}{\ding{51}}%
\newcommand{\xmark}{\ding{55}}%

\newcommand{\hw}[1]{\textcolor{blue}{\textit{HW: #1}}}
\renewcommand{\listingscaption}{Code}

\usepackage[pagebackref,breaklinks,colorlinks]{hyperref}
\setminted[python]{breaklines, framesep=2mm, fontsize=\footnotesize, numbersep=5pt}

\usepackage[capitalize]{cleveref}
\crefname{section}{Sec.}{Secs.}
\Crefname{section}{Section}{Sections}
\Crefname{table}{Table}{Tables}
\crefname{table}{Tab.}{Tabs.}

\def\cvprPaperID{4764} %
\def\confName{CVPR}
\def\confYear{2023}


\begin{document}
\onecolumn
\title{Logical Consistency and Greater Descriptive Power for Facial Hair Attribute Learning}

\author{Haiyu Wu$^{1}$, Grace Bezold$^{1}$, Aman Bhatta$^{1}$, Kevin W. Bowyer$^{1}$\\
$^{1}$University of Notre Dame\\}

\maketitle
\noindent
This supplementary material provides: a)  statistical information for the attributes, b) examples of 28 categories, c) the consistency estimation table and analysis, d) the positive accuracy and negative accuracy on each facial hair attribute, e) logically inconsistent prediction detection f) part of the training and testing code in Code~\ref{code:train} and Code~\ref{code:test}, and g) the facial hair area based demographic analysis on recognition accuracy across Asian male (AM) and Indian male (IM).

\input{Tables/supplemental_material_number_of_samples}

\input{Tables/sup_mat_consistency_rate}

\noindent
\textbf{Statistic information of the attributes:} Table~\ref{sup_table:number_of_samples} shows the number of positive samples of each attribute. Due to the particularity of some attributes, e.g. long beard and bald, it is hard to collect  samples for a balanced number of positive and negative samples. For example, we only find 59 samples that are clearly Bald Sides Only from 608,184 images in the WebFace260M dataset. Since the dataset distributes is a long-tail pattern, the attributes are in a fine-grained level, and the most important is the robustness of the annotations is promised, this dataset has a great potential for use in other research areas.


\noindent
\textbf{Samples of the 28 categories:} Figure~\ref{fig:beard_area} to Figure~\ref{fig:partial_info_not_visible} indicates that the attributes in the FH37K dataset are able to cover the most real-world cases, e.g. occlusion, blurriness, various head poses and lighting angle, etc., on facial hair attributes. Moreover, the pattern of how we design the attributes can be used for future dataset creation.

\noindent
\textbf{Consistency rate estimation:} 
The overall consistency rate is 94.05\%. Table~\ref{sup_table:consistency_rate} gives the estimated consistency rate on each attribute. Consistency occurs in two main situations: edge cases of two attributes, and low image quality. The edge cases usually happen between (Chin Area, Side to Side), (5 O'clock Shadow, Short), (Short, Medium), (Medium, Long). It is hard to make a definition to differentiate the edge images within these pairs, because it could be caused by  head pose, ratio of the face area in the image, etc. Since the images are in-the-wild, the quality of the images cannot be controlled, which is a key factor that increases the consistency for all the annotations. Especially for those connectedness-related attributes: Mustache Connected to Beard, Mustache-Isolated, Sideburns Connected to Beard, and Sideburns-Present. These two situations cause the high consistency rate on: Short (83\%), Medium (89\%), Mustache-Isolated (84\%), Mustache Connected to Beard (83\%), and Sideburns Connected to Beard (90\%).

\noindent
\textbf{Positive accuracy and negative accuracy on each facial hair attribute:} 
Table~\ref{sup_table:performance} shows the performance of our approach - BCELoss + LCPLoss + label compensation strategy - on the logically inconsistent predictions counted cases. Due to the unbalanced number of positive and negative data, the model performs differently on negative and positive side, especially for Bald Sides Only - 98.57 on negative, 0 on positive. There has been a number of research papers that aim to solve this problem, but to our best knowledge, none of them also considers the logical consistency of predictions. Therefore, it is a new challenge that we will continue to investigate in the future.

\input{Tables/sup_mat_accuracy}

\input{Tables/sup_mat_BUPT-B.tex}
\input{Image_tex/arcface_BA-test.tex}
\input{Image_tex/arcface_BUPT-B.tex}
\input{Image_tex/magface_BUPT-B.tex}
\input{Algorithm/logic_relationships.tex}
\input{Image_tex/sup_mat/Beard_area}
\input{Image_tex/sup_mat/Beard_Length}
\input{Image_tex/sup_mat/Mustache}
\input{Image_tex/sup_mat/Side2Side}
\input{Image_tex/sup_mat/Bald}
\input{Image_tex/sup_mat/BA_VIS_INV}

\input{Algorithm/Training_algorithm}

\end{document}
